# Supplementary material for: Outward Influence and Cascade Size Estimation in Billion-scale Networks
Source: arXiv:1704.04794 source file (2017-04-16)
Supplement: Supplementary file 1 [file appendix.tex]

%\appendix
%Let $R_1, R_2, R_3,\ldots, R_j,\ldots$ be the random RR sets generated in either \PIMA{} or \DPIMA{} algorithms.  Given a subset of nodes $S \subset V$, we define   $Z_j = \min\{|R_j \cap S|,1\}$, the Bernouli random variable with mean $\E[Z_j]=\I(S)/n$. Further, define $Y_j = Z_j - \E[Z_j]$, then 
%$Y_j$ is a \emph{martingale} \cite{Chung06}, i.e., $\E[Y_i | Y_1, Y_2,\ldots,Y_{i-1}] = Y_{i-1}$ and $\E[Y_i]<+\infty$.  
%
%This martingale view of $Y_j$ is adopted from \cite{Tang15} to cope with the fact that  $Y_j$ might not be independent due to the stopping condition. Follows \cite{Tang15}, we can obtain the same results in Corollaries 1 and 2 in \cite{Tang15}.
%
%	\begin{Lemma}[\cite{Tang15}]
%	\label{lem:chernoff}
%	Given a set of nodes $S$ and random RR sets $\R = \{R_j\}$ generated in either \PIMA{} or \DPIMA{}, let $Z_1, Z_2,...$ be random variables defined as 
%	\begin{align}
%		Z_j = \left\{ \begin{array}{ll}
%			1 & \text{ if } R_j \cap S \neq \emptyset, \\
%			0 & \text{ otherwise}.
%		\end{array}
%		\right.
%	\end{align}
%	Denote by $\mu_Z$ and  $\sigma_Z^2$ the mean and variance of $Z_j$, respectively. Let $\hat \mu_Z = \frac{1}{T}\sum_{i=1}^{T}Z_i$ be an estimation of $\mu_Z$, for any fixed $T > 0$, and $0 \leq \epsilon \leq 1$, the following inequalities hold,
%	\vspace{-0.05in}
%	\begin{align}
%		\label{eq:plus}
%		\Pr[\hat \mu \geq  (1+ \epsilon) \mu]  \leq
%		e^{\frac{-T\mu\epsilon^2}{2 + \frac{2}{3}\epsilon}},
%	\end{align}
%	\vspace{-0.2in}
%	
%	\noindent and
%	\vspace{-0.05in}
%	\begin{align}
%		\label{eq:minus}
%		\Pr[\hat \mu \leq  (1- \epsilon) \mu] \leq e^{\frac{-T\mu\epsilon^2}{2}}.
%	\end{align}
%	\label{lem:error_bound}
%	\vspace{-0.15in}
%	\end{Lemma}
%    
%    \subsection*{Proof of Lemma~\ref{lem:zo}}
%    This lemma states two properties 1) $\hat \mu_Z$ is an $(\epsilon,\delta)$-approximation   and 2) the (asymptotically) optimal number of samples required $T \leq \textsf{c}_1 \theta^*$. The $(\epsilon,\delta)$-approximation follows directly from Lemma~\ref{lem:chernoff} by applying Eq.~\ref{eq:plus} and Eq.~\ref{eq:minus} to obtain two sides of the desired approximation.
%    
%    To prove the (asymptotic) optimality in terms of the number of samples, we rely on the \textit{Lower Bound Theorem} in \cite{Dagum00}. Lower Bound Theorem states the minimum number of samples $\theta^*$ to achieve an $(\epsilon,\delta)$-approximation given $\epsilon,\delta$,
%    \begin{align}
%    	\theta^* \geq \textsf{c}\Upsilon(\epsilon,\delta/2)\rho_Z/\mu_Z^2 
%    \end{align}
%    where $\rho_Z = \max\{\sigma_Z^2,\epsilon\mu_Z\}$.
%    
%    Thus,
%    \begin{align}
%	    \label{eq:lemzo_1}
%    	\theta^* \frac{\mu_Z}{\textsf{c}\rho_Z} \geq \Upsilon(\epsilon,\delta/2)/\mu_Z = T
%    \end{align}
%    
%  If $\mu_Z \leq 1- \epsilon$, then $\rho_Z = (1 - \mu_Z)\mu_Z$. Eq.~\ref{eq:lemzo_1} is, then, reduced to
%    \begin{align}
%    	T \leq \theta^* \frac{1- \mu_Z}{\textsf{c}  \mu_Z} \leq \theta^* \frac{1}{\textsf{c}}.
%    \end{align}
%    
%    Let $\textsf{c}_1 = \frac{1}{\textsf{c}}$, we achieve,
%    \begin{align}
%    	T \leq \textsf{c}_1\theta^*
%    \end{align}
%
%	\subsection*{Proof of Theorem~\ref{theo:type1}}
%		According to Def.~\ref{def:type1}, if the number of RR sets generated $|\R| \geq N(\epsilon_a, \epsilon_b, \delta_a, \delta_b)$ then Eqs.~\ref{eq:sk} and~\ref{eq:sk*} hold. From Eq.~\ref{eq:sk}, we have,
%		\begin{align}
%		\Pr[\hat \I(\hat S_k) \leq (1 + \epsilon_a) \I(\hat S_k)] \geq 1 - \delta_a
%		\end{align}
%		\noindent which is equivalent to
%		\begin{align}
%		\label{eq:5}
%		\Pr[\I(\hat S_k) \geq \hat \I(\hat S_k) - \epsilon_a\I(\hat S_k)  ] \geq 1 - \delta_a
%		\end{align}
%		Let $S_{kmax} \in V$ be the size-$k$ node set with maximum coverage in $\R$. The greedy strategy in finding max-coverage returns the set, $\hat S_k$, with $\hat \I(\hat S_k) \geq (1 - 1/e)\hat \I(S_{kmax})$ \cite{Nemhauser81}. Since $\hat \I(S_{kmax}) \geq \hat \I(S^*_k)$, $\hat \I(\hat S_k) \geq (1 - 1/e)\hat \I(S^*_k)$. Thus,
%		\begin{align}
%		\Pr[\I(\hat S_k) \geq (1 - 1/e)\hat \I(S^*_{k}) - \epsilon_a\I(\hat S_k)  ] \geq 1 - \delta_a \nonumber
%		\end{align}
%		\noindent Now by substituting $\hat \I(S^*_k)$ in this equation with that from Eq.~\ref{eq:sk*} and noting that the right hand side is updated to $1-\delta_a -\delta_b \geq 1-\delta$ to account for the probability in Eq.~\ref{eq:sk*}. Hence,
%		\begin{align}
%		\Pr[\I(\hat S_k) \geq (1 - 1/e)(1 - \epsilon_b)OPT_k - \epsilon_a\I(\hat S_k)  ] \geq 1 - \delta \nonumber
%		\end{align}
%		\noindent Since $\I(\hat S_k) \leq OPT_k$,
%		\begin{align}
%		\Pr[\I(\hat S_k) \geq (1 - 1/e)(1 - \epsilon_b)OPT_k - \epsilon_aOPT_k  ] \geq 1 - \delta \nonumber
%		\end{align}		
%		\noindent or,
%		\begin{align}
%		\Pr[\I(\hat S_k) \geq (1 - 1/e - (1 - 1/e)\epsilon_b - \epsilon_a)OPT_k  ] \geq 1 - \delta \nonumber
%		\end{align}
%		\noindent and, finally, due to $\epsilon \geq \epsilon_a + (1-1/e)\epsilon_b$,
%		\begin{align}
%		\Pr[\I(\hat S_k) \geq (1 - 1/e - \epsilon)OPT_k  ] \geq 1 - \delta \nonumber
%		\end{align}
%		\noindent That completes the proof of Theo. \ref{theo:type1}.
%%	\end{proof}
%	
%	
%	\textit{Remark}: As shown in \cite{Tang14}, the number of RR sets represent the complexity of an \RIS{} based method. Let $KPT$ be the expected time to generate an RR set, then $|\R|KPT$ is the complexity of generating all the RR sets. Moreover, the finding Max-coverage step can be done in linear time w.r.t the total size of RR sets which is upper-bounded by the generating RR sets which is $|R|KPT$. Thus, we are most interested in \textit{Sample Complexity}.
%	
%	\subsection*{Proof of Lemma~\ref{cor:check}}
%	
%	To prove this lemma, we rely on another result in \cite{Dagum00}.
%	
%	Let $\theta^*, \mu_Z$ be defined as in Lem.~\ref{lem:zo} and $T$ be the number of samples at which $\Cov(Z) \geq 1 + (1 + \epsilon)\Upsilon(\epsilon,\delta/2)$, then $\hat \mu_Z$ is an $(\epsilon, \delta)$-approximation of $\mu_Z$ and, under the realistic assumption that $\mu_Z \leq 1 - \epsilon$, we further have $T \leq (1+\epsilon)\textsf{c}_1\cdot \theta^*$ where $\textsf{c}_1$ is the constant in Lem.~\ref{lem:zo}.
%		
%	Note that if only one side of the $(\epsilon,\delta)$-approximation is required, then $\Upsilon(\epsilon,\delta/2)$ becomes
%	\begin{align}
%		\label{eq:zo_side}
%		\Upsilon(\epsilon,\delta) = (2+\frac{2}{3}\epsilon) \ln \frac{1}{\delta} \frac{1}{\epsilon^2}
%	\end{align}
%	
%	Thus, Lemma~\ref{cor:check} is simply a direct corollary of the above result \cite{Dagum00}.
%	
%	\subsection*{Proof of Lemma~\ref{lem:com1}}
%%	\begin{proof}
%		Recall that $\PIMA{}$ terminates when the selected seed set, $\hat S_k$, satisfies two conditions,
%		\begin{align}
%			\label{eq:con1}
%			\Cov_{\R}(\hat S_k) \geq \Lambda_1
%		\end{align}
%		\vspace{-0.2in}
%		
%		\noindent and
%		\vspace{-0.05in}
%		\begin{align}
%			\label{eq:con2}
%			\hat \I(\hat S_k) \leq (1 + \epsilon_1)\I_c(\hat S_k)
%		\end{align}
%		From Corollary \ref{cor:check}, we have,
%		\begin{align}
%			\label{eq:col1}
%			\Pr[\I_c(S) \leq (1 + \epsilon_2)\I(S)] \geq 1 - \delta/6 \log_2 n
%		\end{align}
%		\noindent Substitute $\I_c(\hat S_k)$ in Eq.~\ref{eq:col1} with that of Eq.~\ref{eq:con2},
%		\begin{align}
%			\label{eq:prob_fail}
%			\Pr[\hat \I(\hat S_k) \leq (1 + \epsilon_{12})\I(\hat S_k)] \geq 1 - \delta/6 \log_2 n
%		\end{align}
%		However, besides the estimation for the final solution $\hat S_k$, we also require all the previous estimations for other candidate solutions returned by \textsf{Estimate-Inf} to be close to true values. Thus, the failure probability in estimating the returned $\hat S_k$ is accumulated from all the influence estimations. In addition, since we start with $\Lambda_1$ RR sets and need the maximum of $(2+\frac{2\epsilon}{3})n \frac{\ln \frac{2}{\delta}+\ln {n\choose k}}{k\epsilon^2}$ (Line 11 in Alg.~\ref{alg:main}), the number of times we need to double the sample size is at most \[
%         \log_2 \frac{n}{k} \left(1+\frac{\ln {n\choose k}}{\ln \frac{2}{\delta}}\right) \leq 2 \log_2 n.
%        \] Hence, combined with Eq.~\ref{eq:prob_fail}, the accumulated failure probability is followed,
%		\begin{align}
%			\Pr[\hat \I(\hat S_k) \leq (1 + \epsilon_{12})\I(\hat S_k)] \geq 1 - \delta/3
%		\end{align}
%		This completes the proof of Lem. \ref{lem:com1}.
%		
%%	\end{proof}
%	
%	\subsection*{Proof of Lemma~\ref{lem:com2}}
%%	\begin{proof}
%		To prove the lemma, we first find a lower-bound of the number of RR sets, $|\R|$, generated and, thus, show that $|\R| \geq \frac{\Upsilon(\epsilon_3,\delta/3) n}{OPT_k}$ with high probability and, then, apply inequalities in Lem.~\ref{lem:chernoff}. Recall that
%		\begin{align}
%		\hat \I(\hat S_k) = \frac{\Cov_{\R}(\hat S_k) n}{|\R|}
%		\end{align}
%		\noindent Apply the first stopping condition, $\Cov_{\R}(\hat S_k) \geq \Lambda_1$,
%		\begin{align}
%		\hat \I(\hat S_k) \geq \frac{\Lambda_1 n}{|\R|} = \frac{(1 + \epsilon_1)(1 + \epsilon_2) \Upsilon(\epsilon_3,\delta/3) n}{|\R|} \nonumber
%		\end{align}
%		\noindent where $\Upsilon(\epsilon_3,\delta/3) = (2+\frac{2}{3}\epsilon_3)\ln (\frac{3}{\delta})\frac{1}{\epsilon_3^2}$.\\
%		
%		Now, combine the result of Lem.~\ref{lem:com1} with the above inequality, we have
%		\begin{align}
%		\Pr[\frac{\Upsilon(\epsilon_3,\delta/3) n}{|\R|} \leq \I(\hat S_k)] \geq 1-\delta/3 \nonumber
%		\end{align}
%		\noindent Thus,
%		\begin{align}
%		\Pr[|\R| \geq \frac{\Upsilon(\epsilon_3,\delta/3) n}{\I(\hat S_k)}] \geq 1-\delta/3
%		\end{align}
%		\noindent and due to $\I(\hat S_k) \leq OPT_k$,
%		\begin{align}
%		\label{eq:num_sam}
%		\Pr[|\R| \geq \frac{\Upsilon(\epsilon_3,\delta/3) n}{OPT_k}] \geq 1-\delta/3
%		\end{align}
%		Eq.~\ref{eq:num_sam} says that $|\R| \geq \frac{\Upsilon(\epsilon_3,\delta/3) n}{OPT_k}$ with at least $(1-\delta/3)$-probability. In cases that $|\R| \geq \frac{\Upsilon(\epsilon_3,\delta/3) n}{OPT_k}$ happens, we use Lem.~\ref{lem:chernoff} on the optimal solution, $S^*_k$, with random variable $Z = \min\{1,|R_j \cap S^*_k|\}$ and $\mu_Z = OPT_k/n$ to obtain
%		\begin{align}
%		\Pr [\hat \I(S^*_k)\leq (1 - \epsilon_3)OPT_k] \leq e^{-\frac{|\R| OPT_k\epsilon^2_3}{n (2+\frac{2}{3}\epsilon_3)}}
%		\end{align}
%		\noindent Then, due to $|\R| \geq \frac{\Upsilon(\epsilon_3,\delta/3) n}{OPT_k}$,
%		\vspace{-0.05in}
%		\begin{align}
%		\label{eq:num_sam_sup}
%		\Pr [\hat \I(S^*_k)\leq (1 - \epsilon_3)OPT_k] \leq e^{-\frac{\Upsilon(\epsilon_3,\delta/3)\epsilon^2_3}{(2+\frac{2}{3}\epsilon_3)}} = \delta/3
%		\end{align}
%		\noindent Thus, combining Eq.~\ref{eq:num_sam} and Eq.~\ref{eq:num_sam_sup} gives
%		\begin{align}
%		\Pr [& \hat \I(S^*_k)\leq (1 - \epsilon_3)OPT_k \text{ or } \hat \I(\hat S_k) \geq (1 + \epsilon_{12})\I(\hat S_k)] \leq 2\delta/3 \nonumber
%		\end{align}
%		%	Accumulate the probabilities of failing when applying Lem. \ref{lem:com1} to bound the number of hyperedges and the above Chernoff-Hoeffding's inequality, we achieve
%		%	\begin{align}
%		%		\Pr [\hat \I(S^*_k)\geq (1 - \epsilon_3)OPT_k] \geq 1 - \delta \nonumber
%		%	\end{align}
%		\noindent which completes the proof of Lem. \ref{lem:com2}.
%%	\end{proof}
%	
%	\subsection*{Proof of Lemma~\ref{lem:num_1}}
%%	\begin{proof}
%		From Lem.~\ref{lem:zo}, to achieve the approximation described in Eq.~\ref{eq:eq2}, we need at least $\frac{\Upsilon(\epsilon_b,\delta_b) n}{OPT_k}$ and
%		\begin{align}
%		\frac{\Upsilon(\epsilon_b,\delta_b) n}{OPT_k} \leq \textsf{c}_1\cdot \theta^*
%		\end{align}
%		\noindent Since $\theta^*$ is the sufficient number of RR sets to achieve Eq.~\ref{eq:eq1} only and $N^1_{min}(\epsilon_a,\epsilon_b,\delta_a,\delta_b)$ is enough to obtain both Eq.~\ref{eq:eq1} and Eq~\ref{eq:eq2}, we get $\theta^* \leq N^1_{min}(\epsilon_a,\epsilon_b,\delta_a,\delta_b)$ and, thus,
%		\begin{align}
%		\frac{\Upsilon(\epsilon_b,\delta_b) n}{OPT_k} \leq \textsf{c}_1\cdot N^1_{min}(\epsilon_a,\epsilon_b,\delta_a,\delta_b)
%		\end{align}
%		\noindent Multiply both sides by $\frac{1}{1-1/e-\epsilon}$,
%		\begin{align}
%		\frac{\Upsilon(\epsilon_b,\delta_b) n}{(1-1/e-\epsilon)OPT_k} \leq \frac{\textsf{c}_1\cdot N^1_{min}(\epsilon_a,\epsilon_b,\delta_a,\delta_b)}{1-1/e-\epsilon}
%		\end{align}
%		\noindent Since $\I(\hat S_k)\geq (1-1/e-\epsilon)OPT_k$, we have
%		\begin{align}
%		\label{eq:eq3}
%		\frac{\Upsilon(\epsilon_b,\delta_b) n}{\I(\hat S_k)} \leq \frac{\textsf{c}_1\cdot N^1_{min}(\epsilon_a,\epsilon_b,\delta_a,\delta_b)}{1-1/e-\epsilon}
%		\end{align}
%		Recall that $\hat \I(\hat S_k) = \frac{\Cov_{\R}(\hat S_k)n}{|\R|}$ or $|\R| = \frac{\Cov_{\R}(\hat S_k)n}{\hat \I(\hat S_k)}$. Thus, the condition $\Cov_{\R}(\hat S_k) \geq \Lambda_1$ is equivalent to
%		\begin{align}
%		\label{eq:eq4}
%		|\R| \geq \frac{\Lambda_1 n}{\hat \I(\hat S_k)} = \frac{(1+\epsilon_a)\Upsilon(\epsilon_b,\delta_b) n}{\hat \I(\hat S_k)}
%		\end{align}
%		\noindent Since $\hat \I(\hat S_k) \leq (1 + \epsilon_a)\I(\hat S_k)$, we also have
%		\begin{align}
%		\label{eq:eq6}
%		\frac{\Upsilon(\epsilon_b,\delta_b) n}{\I(\hat S_k)} \leq \frac{(1+\epsilon_a)\Upsilon(\epsilon_b,\delta_b) n}{\hat \I(\hat S_k)}
%		\end{align}
%		From Eq.~\ref{eq:eq4} and Eq.~\ref{eq:eq6}, observe that if we set $|\R| = \frac{\Upsilon(\epsilon_b,\delta_b) n}{\I(\hat S_k)}$ then Eq.~\ref{eq:eq4} will hold and, in turn, we achieve $\Cov_{\R}(\hat S_k) \geq \Lambda_1$. Based on that and Eq.~\ref{eq:eq3}, we conclude that $\frac{\textsf{c}_1\cdot N^1_{min}(\epsilon_a,\epsilon_b,\delta_a,\delta_b)}{1-1/e-\epsilon}$ RR sets are sufficient to satisfy the condition (\ref{eq:c1}).
%		%	\noindent Moreover, due to the doubling RR sets scheme in each iteration and the fact that \PIMA{} stops whenever Eq.~\ref{eq:eq4} is satisfied, we have
%		%	\vspace{-0.1in}
%		%	\begin{align}
%		%	\label{eq:eq5}
%		%	|\R| \leq 2\frac{\Upsilon_3 n}{\I(\hat S_k)}
%		%	\end{align}
%		%	\vspace{-0.2in}
%		%	
%		%	Thus, combining Eq. \ref{eq:eq3} and Eq. \ref{eq:eq5}, we get
%		%	\vspace{-0.1in}
%		%	\begin{align}
%		%	|\R| \leq \frac{2\textsf{a} }{1-1/e-\epsilon}\theta^*(\epsilon_1+\epsilon_2+\epsilon_1\epsilon_2,\epsilon_3,\delta/2,\delta/2)
%		%	\end{align}
%		%	\vspace{-0.2in}
%%	\end{proof}
%	
%	
%	\subsection*{Proof of Lemma~\ref{lem:num_2}}
%%	\begin{proof}
%		In this case, the necessary number of RR sets is the same as that to satisfy Eq.~\ref{eq:eq1} where $\epsilon_a = \epsilon_1 + \epsilon_2 + \epsilon_1\epsilon_2$. The only question here is whether the \textsf{Estimate-Inf} succeeds and returns $\I(\hat S_k)$ when the main algorithm has $|\R|$ random RR sets. Recall that it fails in the case that the number of RR sets required in \textsf{Estimate-Inf} exceeds $2|\R|\frac{1 + \epsilon_2}{1-\epsilon_2}\frac{\epsilon_3^2}{\epsilon_2^2}$, however, from Eq.~\ref{eq:eq3},
%		\begin{align}
%			|\R| \geq \frac{\Upsilon(\epsilon_b,\delta_b) n}{\I(\hat S_k)} = (2+\frac{2}{3}\epsilon_3)\ln \frac{3}{\delta} \frac{1}{\epsilon_3^2} \frac{n}{\I(\hat S_k)}
%		\end{align}
%		\noindent Multiply both side with $2\frac{1 + \epsilon_2}{1-\epsilon_2}\frac{\epsilon_3^2}{\epsilon_2^2}$,
%		\begin{align}
%			\label{eq:check_sam}
%			2|\R|&\frac{1 + \epsilon_2}{1-\epsilon_2}\frac{\epsilon_3^2}{\epsilon_2^2} \geq 2\frac{1 + \epsilon_2}{1-\epsilon_2} (2+\frac{2}{3}\epsilon_3)\ln \frac{3}{\delta} \frac{1}{\epsilon_2^2} \frac{n}{\I(\hat S_k)} \nonumber \\
%			&\geq \frac{1 + \epsilon_2}{1-\epsilon_2} (2+\frac{2}{3}\epsilon_3) (\ln \frac{3}{\delta}+\ln[2 \log_2 n]) \frac{1}{\epsilon_2^2} \frac{n}{\I(\hat S_k)}
%		\end{align}
%		The last inequality is due to our practical assumption that $3/\delta \geq 2\log_2 n$. Based on Lem.~\ref{lem:zo}, with $(2+\frac{2}{3}\epsilon_3)(\ln \frac{3}{\delta}+\ln[2 \log_2 n]) \frac{1}{\epsilon_2^2} \frac{n}{\I(\hat S_k)}$ random RR sets, it is sufficient to obtain
%		\begin{align}
%			\label{eq:eq11}
%			\Pr\Big[\I_c(\hat S_k) \geq (1-\epsilon_2) \I(\hat S_k)\Big] \leq 1 - \frac{\delta}{6 \log_2 n}
%		\end{align}
%		\noindent Thus, combine Eq.~\ref{eq:check_sam} and Eq.~\ref{eq:eq11},
%		\begin{align}
%			\Pr\Big[2|\R|\frac{1 + \epsilon_2}{1-\epsilon_2}\frac{\epsilon_3^2}{\epsilon_2^2} & \geq (1+\epsilon_2) (2+\frac{2}{3}\epsilon_3)(\ln \frac{3}{\delta} \nonumber \\ &+\ln[2 \log_2 n]) \frac{1}{\epsilon_2^2} \frac{n}{\I_c(\hat S_k)}\Big] \leq 1 - \frac{\delta}{6 \log_2 n} \nonumber
%		\end{align}
%		\noindent or,
%		\begin{align}
%			\Pr\Big[\frac{\I_c(\hat S_k)}{n}2|\R|\frac{1 + \epsilon_2}{1-\epsilon_2}\frac{\epsilon_3^2}{\epsilon_2^2} & \geq (1+\epsilon_2) (2+\frac{2}{3}\epsilon_3) (\ln \frac{3}{\delta} \nonumber \\
%			&+ \ln [2\log_2 n]) \frac{1}{\epsilon_2^2}\Big] \geq 1 - \frac{\delta}{6 \log_2 n} \nonumber
%		\end{align}
%		\noindent The left hand side, $\frac{\I_c(\hat S_k)}{n}2|\R|\frac{1 + \epsilon_2}{1-\epsilon_2}\frac{\epsilon_3^2}{\epsilon_2^2}$, is the coverage, $\Cov$, in \textsf{Estimate-Inf} procedure when $2|\R|\frac{1 + \epsilon_2}{1-\epsilon_2}\frac{\epsilon_3^2}{\epsilon_2^2}$ RR sets are generated and the whole inequality is the condition to succeed. That means with $|\R|$ RR sets in the main algorithm, the \textsf{Estimate-Inf} returns a good estimation of $\I(\hat S_k)$ with at least $(1-\delta/3)$-probability.
%%	\end{proof}
%	
%	\subsection*{Proof of Lemma~\ref{lem:epsilon_dima}}
%%	\begin{proof}
%		To prove the lemma, we begin by showing that $\I(S^*_k)$ has an better approximation when $|\R| \geq M\textsf{c}_1N^2_{min}(\epsilon, \delta)$. Let $X^* = \min\{1, |R_j \cap S^*_k|\}$ ($R_j$ is a random RR set) be a random variable with $\mu_{X^*} = OPT_k/n$. Apply Lem.~\ref{lem:zo} on the approximation of $\mu_{X^*}$ to achieve Eq.~\ref{eq:given2}, we have
%		\begin{align}
%		\frac{\Upsilon(\epsilon^*_b,\delta^*_b)}{\mu_{X^*}} \leq \textsf{c}_1 N^2_{min}(\epsilon, \delta)
%		\end{align}
%		%		
%		%		\noindent or, equivalently,
%		%		\vspace{-0.1in}
%		%		\begin{align}
%		%			2c\ln\frac{1}{\delta^*_b}\frac{n}{\epsilon^{*2}_b OPT_k} \leq \textsf{c}_1 \Theta^*(\epsilon,\delta)
%		%		\end{align}
%		%		\vspace{-0.15in}
%		\noindent Multiplying both sides by $M$ gives
%		\begin{align}
%		\frac{M\Upsilon(\epsilon^*_b,\delta^*_b)}{\mu_{X^*}} \leq M\textsf{c}_1N^2_{min}(\epsilon, \delta)
%		\end{align}
%		\noindent In other words,
%		\begin{align}
%		\label{eq:new_set}
%		|\R| \geq \frac{M\Upsilon(\epsilon^*_b,\delta^*_b)}{\mu_{X^*}}
%		\end{align}
%		\noindent Then, since
%		\begin{align}
%		M\Upsilon(\epsilon^*_b,\delta^*_b)=\frac{\ln\frac{2}{\delta^*_b}}{\ln \frac{1}{\delta^*_b}}\frac{8(1+\epsilon)(1+\epsilon^*_a)^2}{(\frac{1}{2}-\frac{1}{e}-\frac{\epsilon}{2})^3} \Upsilon(\epsilon^*_b,\delta^*_b) \geq \Upsilon(\frac{\epsilon^*_b}{2},\frac{\delta^*_b}{2}), \nonumber
%		\end{align}
%		\vspace{-0.2in}
%		
%		\noindent thus,
%		\vspace{-0.05in}
%		\begin{align}
%		\label{eq:new_set_2}
%		|\R| \geq \frac{\Upsilon(\frac{\epsilon^*_b}{2},\frac{\delta^*_b}{2})}{\mu_{X^*}}
%		\end{align}
%		Apply Lem.~\ref{lem:zo} with the number of RR sets specified in Eq.~\ref{eq:new_set_2}, we have
%		\begin{align}
%		\label{eq:eq9}
%		\Pr[\hat \I(S^*_k) \geq (1 - \epsilon^*_b/2)OPT_k] \geq 1 - \delta^*_b/2
%		\end{align}
%		\noindent Combine Eq.~\ref{eq:given1} and Eq.~\ref{eq:eq9} and apply Theo.~\ref{theo:type1},
%		\begin{align}
%		\label{eq:new_approx}
%		\Pr[\I(\hat S_k) \geq (1-\frac{1}{e}-\epsilon)OPT_k] \geq 1-\delta^*_a - \frac{\delta^*_b}{2}
%		\end{align}
%		In Eq. \ref{eq:new_set}, $|\R|$ depends on $\mu_{X^*} = OPT_k/n$ and in Eq. \ref{eq:new_approx}, we obtained the relation between $\I(\hat S_k)$ and $OPT_k$ and, thus, we can represent $|\R|$ in terms of $\I(\hat S_k)$,
%		\begin{align}
%		\Pr[|\R| \geq \frac{M\Upsilon(\epsilon^*_b,\delta^*_b)(1-1/e-\epsilon)}{\I(\hat S_k)/n}] \geq 1-\delta^*_a - \frac{\delta^*_b}{2} \nonumber
%		\end{align}
%		\noindent and since $M\Upsilon(\epsilon^*_b,\delta^*_b)(1-1/e-\epsilon) \geq \Upsilon(\frac{\epsilon^*_b}{2},\frac{\delta^*_b}{2})$,
%		\begin{align}
%		\label{eq:num_rr}
%		\Pr[|\R| \geq \frac{\Upsilon(\frac{\epsilon^*_b}{2},\frac{\delta^*_b}{2})}{\I(\hat S_k)/n}] \geq 1-\delta^*_a - \frac{\delta^*_b}{2}
%		\end{align}
%		%		\begin{align}
%		%			\textsf{a}\cdot \Theta^*(\epsilon,\delta) \geq 2c\ln\frac{2}{\delta^*_b}\frac{n\cdot (1-\epsilon^*_b)}{\epsilon^{*2}_b \hat \I(S^*_k)}
%		%		\end{align}
%		%		\vspace{-0.15in}
%		
%		Notice that in each iteration \DPIMA{} generates $|\R|$ new random RR sets and put them in $\R'$ to compute $\I_c(\hat S_k)$. Thus,
%		\vspace{-0.05in}
%		\begin{align}
%		\label{eq:num_rr'}
%		\Pr[|\R'| \geq \frac{\Upsilon(\frac{\epsilon^*_b}{2},\frac{\delta^*_b}{2})}{\I(\hat S_k)/n}] \geq 1-\delta^*_a - \frac{\delta^*_b}{2}
%		\end{align}
%		\noindent In the cases that $|\R'| \geq \frac{\Upsilon(\frac{\epsilon^*_b}{2},\frac{\delta^*_b}{2})}{\I(\hat S_k)/n}$, apply Lem.~\ref{lem:zo},
%		\begin{align}
%		\Pr[\I_c(\hat S_k) \geq (1 - \epsilon^*_b/2)\I(\hat S_k)] \geq 1 - \delta^*_b/2
%		\end{align}
%		\noindent Combine with the probability in Eq.~\ref{eq:num_rr'}, we have
%		\begin{align}
%		\Pr[\I_c(\hat S_k) \geq (1 - \epsilon^*_b/2)\I(\hat S_k)] \geq 1 - \delta^*_a - \delta^*_b
%		\end{align}
%		\noindent or, equivalently,
%		\begin{align}
%		\label{eq:new_app}
%		\Pr[\I(\hat S_k) \leq \frac{1}{1 - \epsilon^*_b/2}\I_c(\hat S_k)] \geq 1 - \delta^*_a - \delta^*_b
%		\end{align}
%		\noindent Thus, from Eq.~\ref{eq:given1} and Eq.~\ref{eq:new_app} with a note that Eq.~\ref{eq:given1} was used to derive Eq.~\ref{eq:new_app} and, thus, the probability that both happen is actually the probability in Eq.~\ref{eq:new_app}, we achieve
%		\begin{align}
%		\label{eq:eq10}
%		\Pr[\hat \I(\hat S_k) \leq \frac{1 + \epsilon^*_a}{1-\epsilon^*_b/2} \I_c(\hat S_k)] \geq 1 - \delta^*_a - \delta^*_b
%		\end{align}
%		\noindent Then, since $\epsilon_1 = \frac{\hat \I(\hat S_k)}{\I_c(\hat S_k)} -1$ and from Eq.~\ref{eq:eq10},
%		\begin{align}
%		\Pr[\epsilon_1 \leq \frac{1 + \epsilon^*_a}{1 - \epsilon^*_b/2}-1] \geq 1 - \delta^*_a - \delta^*_b
%		\end{align}
%		\noindent and due to $\delta^*_a + \delta^*_b \leq \delta$,
%		\begin{align}
%		\Pr[\epsilon_1 \leq \frac{\epsilon^*_a+\epsilon^*_b/2}{1 - \epsilon^*_b/2}] \geq 1-\delta
%		\end{align}
%		\noindent which completes the proof.
%%	\end{proof}
%\balance	
%	\subsection*{Proof of Lemma~\ref{lem:2}}
%%	\begin{proof}
%		Notice that since $\epsilon \leq 1-2/e$, we have $\frac{\epsilon^*_a+\epsilon^*_b/2}{1 - \epsilon^*_b/2} \leq \epsilon$ and the condition in Line 9 is satisfied. Given $\epsilon_1 \leq \frac{\epsilon^*_a+\epsilon^*_b/2}{1 - \epsilon^*_b/2}$, we compute $\epsilon_2, \epsilon_3$ as,
%		\begin{align}
%		\label{eq:e2}
%		\epsilon_2 = \frac{\epsilon-\epsilon_1}{2(1+\epsilon_1)} \geq \frac{1/2-1/e-\epsilon/2}{1+\epsilon^*_a}\frac{\epsilon^*_b}{2}
%		\end{align}
%		\vspace{-0.2in}
%		
%		\noindent and
%		\begin{align}
%			\label{eq:e3}
%			\epsilon_3 = \frac{\epsilon-\epsilon_1}{2(1-1/e)} \geq (1/2-1/e-\epsilon/2)\frac{\epsilon^*_b}{2}
%		\end{align}
%		Since $\epsilon_1 \leq \frac{\epsilon^*_a+\epsilon^*_b/2}{1 - \epsilon^*_b/2}$ also implies that all the inequality used in the proof of Lem. \ref{lem:epsilon_dima} hold, then
%		\begin{align}
%			\hat \I(S^*_k) \geq (1 - \epsilon^*_b/2)OPT_k
%		\end{align}
%		\noindent Combine with $\hat \I(\hat S_k) \geq (1-1/e)\hat \I(S^*_k)$, we have
%		\begin{align}
%			\hat \I(\hat S_k) \geq (1-1/e)(1 - \epsilon^*_b/2)OPT_k
%		\end{align}
%		\noindent Replace $OPT_k$ in $\mu_{X^*} = OPT_k/n$ by that in the above inequality, we get $\mu_{X^*} \leq \frac{\hat \I(\hat S_k)}{n(1-1/e)(1 - \epsilon^*_b/2)} \leq \frac{\hat \I(\hat S_k)}{n(\frac{1}{2}-\frac{1}{e}-\frac{\epsilon}{2})}$ and then the number of RR sets in Eq.~\ref{eq:new_set} is rewritten as,
%		\begin{align}
%			|\R| \geq \frac{\ln\frac{2}{\delta^*_b}}{\ln \frac{1}{\delta^*_b}}\frac{8(1+\epsilon)(1+\epsilon^*_a)^2}{(\frac{1}{2}-\frac{1}{e}-\frac{\epsilon}{2})^2}\frac{\Upsilon(\epsilon^*_b,\delta^*_b)}{\hat \I(\hat S_k)/n}
%		\end{align}
%		\noindent or, equivalently,
%		\begin{align}
%			\label{eq:base}
%			|\R|\frac{\hat \I(\hat S_k)}{n} &\geq (2+\frac{2}{3}\epsilon_3)\ln \frac{2}{\delta^*_b}\frac{8(1+\epsilon)(1+\epsilon^*_a)^2}{(\frac{1}{2}-\frac{1}{e}-\frac{\epsilon}{2})^2\epsilon^{*2}_b}
%		\end{align}
%		\noindent The left hand side is the coverage of $\hat S_k$ in $\R$, $\Cov_{\R}(\hat S_k)$. Combining that and the calculated $\epsilon_1,\epsilon_2,\epsilon_3$ to find $\delta_1$ with a note that $(1+\epsilon_1)(1+\epsilon_2) \leq (1+\epsilon)$,
%		\begin{align}
%			\label{eq:d1}
%			\delta_1 &= e^{-\frac{\Cov_{\R}(\hat S_k)\cdot \epsilon_3^2}{(2+\frac{2}{3}\epsilon_3)(1+\epsilon_1)(1+\epsilon_2)}} \nonumber \\ &\leq e^{-\frac{(2+\frac{2}{3}\epsilon_3)\ln \frac{2}{\delta^*_b}\frac{8(1+\epsilon)(1+\epsilon^*_a)^2}{(\frac{1}{2}-\frac{1}{e}-\frac{\epsilon}{2})^2\epsilon^{*2}_b}\cdot \epsilon_3^2}{(2+\frac{2}{3}\epsilon_3)(1+\epsilon_1)(1+\epsilon_2)}} \leq \frac{\delta^*_b}{4 \log_2 n} \leq \frac{\delta^*_b}{2}
%		\end{align}
%		To compute the value of $\delta_2$, we base on the fact that $|\R'| = |\R|$ and Eq.~\ref{eq:num_rr'} with a note that $1+\epsilon_2 \leq 1+\epsilon$ and $\ln \frac{2}{\delta^*_b} \geq \ln [2 \log_2 n]$,
%		\begin{align}
%			\label{eq:d2}
%			\delta_2 & = e^{-\frac{\Cov_{\R'}(\hat S_k)\cdot \epsilon_2^2}{(2+\frac{2}{3}\epsilon_3)(1+\epsilon_2)} + \ln [2 \log_2 n]} \nonumber \\
%			&\leq e^{-2\frac{(2+\frac{2}{3}\epsilon_3)\ln \frac{2}{\delta^*_b}\frac{8(1+\epsilon)(1+\epsilon^*_a)^2}{(\frac{1}{2}-\frac{1}{e}-\frac{\epsilon}{2})^2\epsilon^{*2}_b}\cdot \epsilon_2^2}{(2+\frac{2}{3}\epsilon_3)(1+\epsilon_2)} + \ln[2 \log_2 n]} \leq \delta^*_b/2
%		\end{align}
%		From Eq.~\ref{eq:d1} and Eq.~\ref{eq:d2}, we conclude
%		\begin{align}
%			\delta_1 + \delta_2 \leq \delta^*_b/2 + \delta^*_b/2 = \delta^*_b \leq \delta
%		\end{align}
%		\noindent which proves Lem. \ref{lem:2}.
%		%			\vspace{-0.05in}
%		%			\begin{align}
%		%				\label{eq:2}
%		%				\hat \I(\hat S_k) \leq (1 + \epsilon^*_a) \I(\hat S_k)
%		%			\end{align}
%		%			\vspace{-0.15in}
%		%			
%		%			\noindent Replace $\I(\hat S_k)$ in Eq. \ref{eq:1} by that from Eq. \ref{eq:2},
%		%			\vspace{-0.1in}
%		%			\begin{align}
%		%				\label{eq:3}
%		%				|\R| \geq 	\frac{\ln\frac{4}{\delta^*_b}}{\ln \frac{1}{\delta^*_b}}\frac{4(1+\epsilon^*_a)^2}{(\frac{1}{2}-\frac{1}{e}-\frac{\epsilon}{2})^2}\frac{\Upsilon(\epsilon^*_b,\delta^*_b)(1-1/e-\epsilon)}{\I(\hat S_k)/n}
%		%			\end{align}
%		%			\vspace{-0.2in}
%		%			
%		%			
%		%			\noindent Consequently, we can compute $\delta_1$ from $\epsilon_2, \epsilon_3$,
%		%			\vspace{-0.1in}
%		%			\begin{align}
%		%				\delta_1 = e^{-\frac{\Cov_{\R}(\hat S_k)\cdot \epsilon_3^2}{2c(1+\epsilon_1)(1+\epsilon_2)}}
%		%			\end{align}
%		%			\vspace{-0.2in}
%		
%%	\end{proof}
